# Supplementary material for: CWF: Consolidating Weak Features in High-quality Mesh Simplification
Source: arXiv:2404.15661 source file (2024-04-24)
Supplement: Supplementary file 1 [file 9-appendix.tex]

\appendix

\section{Appendix}

\subsection{Original Versions of Organic model}
\XR{Maybe remove.}
Fig.~\ref{fig:Original1} and Fig.~\ref{fig:Original2}
shows the original versions of the organic model from Fig.~1 in the main paper. It can be seen that the original versions of the organic models are heavily smoothed. 
These weak features are prone to being erased during simplification. However, our method showcases the ability to consolidate weak features while maintaining high-quality triangulation.
With this advantageous property,
our algorithm has the potential to convey visual shape clues through a simplified representation.

\begin{figure*}[H]
    \centering
    \begin{overpic}[width=0.93\linewidth]{figures/111.png}
    \put(-3, 20){\rotatebox{90}{\textbf{{Original model}}}}
    \put(-3, 5){\rotatebox{90}{\textbf{{Our result}}}}
    \end{overpic}
    \vspace{0pt}
    \caption{The original versions of the organic models and our results, it is easy to see that the original organic models are heavily smoothed.}
    \label{fig:Original1}
\end{figure*}

\begin{figure}[H]
    \centering
    \begin{overpic}[width=0.93\linewidth]{figures/222.png}
    \put(0, -3){(a) Original model}
    \put(40, -3){(b) Our result}
    \end{overpic}
    \vspace{5pt}
    \caption{The original versions of the organic models and our results, it is easy to see that the original organic models are heavily smoothed}
    \label{fig:Original2}
\end{figure}
